# Supplementary material for: Motif Learning in Knowledge Graphs Using Trajectories Of Differential Equations
Source: arXiv:2010.06684 source file (2020-10-18)
Supplement: Supplementary file 1 [file appendix.tex]

\section{Appendix}

\begin{align*}
 \begin{blockarray}{ccc}
  \begin{block}{c|c|c}
  \boldsymbol{e_1}^{m_1} \circ r  = \boldsymbol{e_2}^{m_1}& &\\ % Row 1
  \end{block}
  \begin{block}{c|c|c}
    \boldsymbol{e_2}^{m_1} \circ r = \boldsymbol{e_3}^{m_1}& \boldsymbol{e_1}^{m_1} \circ r \circ r = \boldsymbol{e_3}^{m_1}, &\\ % Row 2
  \end{block}
    \begin{block}{c|c|c}
    \boldsymbol{e_3}^{m_1} \circ r = \boldsymbol{e_4}^{m_1}& \boldsymbol{e_1}^{m_1} \circ r \circ r \circ r = \boldsymbol{e_4}^{m_1}, &\\ % Row 2
  \end{block}
  \begin{block}{c|c|c}
    \vdots& \vdots\\  % Row 3
  \end{block}
      \begin{block}{c|c|c}
    \boldsymbol{e_9}^{m_1} \circ r = \boldsymbol{e_{10}}^{m_1}& \boldsymbol{e_1}^{m_1} \circ r \dots \circ r = \boldsymbol{e_{10}}^{m_1}, &\\ % Row 2
  \end{block}
  \begin{block}{c|c|c}
    \boldsymbol{e_{10}}^{m_1} \circ r = \boldsymbol{e_1}^{m_1}.& \boldsymbol{e_1}^{m_1} \circ r \dots \circ r = \boldsymbol{e_1}^{m_1}. & r = 1 \rightarrow \theta_{r} = 2\pi/10 \\ % Row 4
  \end{block}
  \end{blockarray}
\end{align*}

\begin{align*}
 \begin{blockarray}{ccc}
  \begin{block}{c|c|c}
  \boldsymbol{e_1}^{m_2} \circ r  = \boldsymbol{e_2}^{m_2}& &\\ % Row 1
  \end{block}
  \begin{block}{c|c|c}
    \boldsymbol{e_2}^{m_2} \circ r = \boldsymbol{e_3}^{m_2}& \boldsymbol{e_1}^{m_2} \circ r \circ r = \boldsymbol{e_3}^{m_2}, &\\ % Row 2
  \end{block}
    \begin{block}{c|c|c}
    \boldsymbol{e_3}^{m_2} \circ r = \boldsymbol{e_4}^{m_2}& \boldsymbol{e_1}^{m_2} \circ r \circ r \circ r = \boldsymbol{e_4}^{m_2}, &\\ % Row 2
  \end{block}
  \begin{block}{c|c|c}
    \vdots& \vdots\\  % Row 3
  \end{block}
      \begin{block}{c|c|c}
    \boldsymbol{e_9}^{m_2} \circ r = \boldsymbol{e_{10}}^{m_2}& \boldsymbol{e_1}^{m_2} \circ r \dots \circ r = \boldsymbol{e_{10}}^{m_2}, & \boldsymbol{e_1}^{m_2} * 20\pi i/10 =  \boldsymbol{e_{10}}^{m_2} * r \\ % Row 2
  \end{block}
  \end{blockarray}
\end{align*}
